# Supplementary material for: The human side of Software Engineering Teams: an investigation of contemporary challenges
Source: arXiv:2104.03712 source file (2022-01-31)
Supplement: Supplementary file 1 [file challenge_changelog.tex]

\section{Changes made to the initial challenge set} \label{appendix_delta}
This is a list of changes that were made to the initial challenges to create the refined problem set, based on feedback in the survey.

The following challenges were \textbf{removed}:
\begin{itemize}
    \item T3 "Lack of teamwork skills", because it was too vague and subject to interpretation.
    \item T4 "Lack of leadership", because it was too vague and could express itself in many ways. The challenges "Lack of mentors", "Lack of mediation in conflict cases", "Demotivation" etc represent the many effects in a more fine-grained manner.
    \item T12 "Insufficient collaboration", because it was too vague.
    \item T17 "Conflicts of interest at management level" because it is too vague, and depending on the interpretation, too close to "Work is not solution-oriented", "Harassment" or "Destructive competition".
    \item T18 "Missing documentation of the project" - not enough of a human challenge. Underlying causes better described with challenges such as T7, T15, T26.
    \item T19 "Information is not made known to the team" - too vague as the challenge depends on who the actor is. It could be missing documentation, bad team coherence, or bad leadership.
    \item T26 "Conflicting working styles" because it was too vague.
    \item T28 "People crying in discussions" removed because it was not seen as relevant in the survey.
\end{itemize}

The following challenges were grouped into a single challenge as they were \textbf{too close in their meaning}:
\begin{itemize}
    \item T6, T25 and T33 merged with T15 "Work is not solution-oriented"
    \item T9, T10, and T11 were merged into one single challenge: "Reluctance to change working habits"
    \item T16 "Language barriers" merged with T20 "Misunderstandings in communication"
    \item T23 "Missing acceptance of alternative lifestyles" merged with T24 "Harassment"
    \item T27 "People getting angry in discussions" merged with new challenge "Aggressive Discussion Styles"
\end{itemize}

The following challenges were \textbf{refined} in their wording:
\begin{itemize}
    \item "Communication plan is neglected" reworded to "Team is not kept up-to-date", as the "plan" specialization is overly specific and other communication issues are better covered by other challenges (such as "Discussions are not solution-oriented").
    \item "Insufficient analysis at the beginning of the task" reworded to "Tasks insufficiently analyzed", to focus more on the actual challenge and remove the temporal component.
    \item "Subjective interpretation of tasks" reworded to "Task is not well defined or explained".
    \item "Misunderstandings in communication" reworded to "Misunderstandings" as it should also cover documentation and anything conveyed via words.
    \item "Certain people dominating discussions" reworded to "Aggressive Discussion Styles" to cover more general discussion issues caused by forceful or aggressive behaviour.
    \item "Missing respect in the workplace" reworded to "Missing appreciation" to distance it from "Harassment" and cover a new aspect.
    \item T32 "Pressure from client forwarded to SE team" generalised to any kind of "Pressure".
\end{itemize}

The following challenges were \textbf{added based on feedback} from the survey:
\begin{itemize}
    \item Different communication preferences
    \item Destructive Competition
    \item Lack of Empathy
    \item Negativity
    \item Lack of mentors
    \item Lack of mediation in conflicts
    \item Bad Work-Life-Balance
    \item Lack of Confidence
    \item Missing team cohesion
    \item Different needs of staff not respected
\end{itemize}
