# Supplementary material for: The human side of Software Engineering Teams: an investigation of contemporary challenges
Source: arXiv:2104.03712 source file (2022-01-31)
Supplement: Supplementary file 2 [file challenge_descriptions.tex]

\section{Challenge Descriptions} \label{appendix_challdesc}
\subsection{Interpersonal Challenges}
1. \textbf{“Not my job”-mentality}\newline
People that refuse to take on or help with tasks that are outside of their role or were not explicitly assigned to them during the planning process. Includes situations in which team members stumble across an issue that was not their responsibility, but they could fix with relative ease, yet they choose not to.

2. \textbf{Different communication preferences}\newline
Clashing preferences of how synchronization should happen (chat, mail, voice calls, video calls, in-person meetings, via documentation/planning tools) leading to people being upset over the chosen mode or planning being delayed or obstructed due to unmotivated participation.

3. \textbf{Destructive Competition}\newline
People that put their own personal gain above the common goal. Prestigious tasks are not assigned to the most competent person but out of political reasons. (Representatives of ) departments refusing to cooperate or even manipulating others to profit personally.

4. \textbf{Under-Estimation of skills}\newline
People that systematically underestimate their potential, thus avoiding challenging tasks and potentially limiting their own growth.

5. \textbf{Over-Estimation of skills}\newline
People that systematically overestimate their current skill and knowledge, leading to incorrect time or budget estimates.

6. \textbf{Lack of Empathy}\newline
People without a sense of how those around them feel or without a will to adapt to the emotional state of colleagues. Example: Anxious colleague is yelled at for not being able to complete a task instead of supported. Emotional unrest is not recognized and no support offered by superiors or colleagues.

7. \textbf{Pressure}\newline
People being pressured to be more productive using forceful communication  (yelling, belittling, needlessly pointing out deadlines) instead of jointly looking for ways or getting additional resources to improve the situation.

8. \textbf{People not reporting problems in time}\newline
People not requesting assistance or not reporting a blocking problem immediately, potentially pretending there is no problem as to not lose face, potentially endangering financial or time constraints.

9. \textbf{Frequently changing team members}\newline
The teams are often recomposed and workers have to work with and adapt to new team members.

10. \textbf{Aggressive Discussion Styles}\newline
People that use shouting, yelling and general aggressive verbal modes, or try to allocate a lot of speaking time for themselves, while not giving room to speak for less dominant colleagues.

11. \textbf{Misunderstandings}\newline
The intended meaning is not transferred accurately over the selected communication channel. This could be due to bad pronunciation, language barriers, technical issues, use of sarcasm/irony, leaving out details because it is assumed it is already known etc.

12. \textbf{Discussions are not solution-oriented}\newline
Discussions or meeting often either become off-topic or are not aimed towards finding an actual solution, but rather used as a vent to complain about circumstances.

13. \textbf{Reluctance to change working habits}\newline
Staff are reluctant to try out new infrastructure, processes or tools and would rather stick to the established, even if it is known to perform worse.

14. \textbf{Team is not kept up-to-date}\newline
Updates regarding the project, the team’s or company’s vision, problems and goals or staff changes are not communicated clearly and in time. 

15. \textbf{Lack of mentors}\newline
Delays occur as there is no designated person to contact in case of technical issues or lack of knowledge about company procedures.

16. \textbf{Missing team cohesion}\newline
There is no feeling of being a “closely knit” team, with its members supporting each other technically and emotionally and being interested in each other’s tasks.

17. \textbf{Different needs of staff not respected}\newline
The working environment does not cater to individual needs and requests for individual changes are not respected by the management, leading to colleagues feeling unhappy about the place they work in. Examples: Standing desks are denied. People are forced to work in open space offices.

18. \textbf{Negativity}\newline
A general sense of negativity lingers, causing demotivation and rants rather than a productive spirit of problem solving.

19. \textbf{Harassment}\newline
People harassing colleagues, including insults, threats, belittling, lack of respect, racism and sexism. 

20. \textbf{Missing appreciation}\newline
Superiors or colleagues rarely acknowledge the work behind a successful task, or the sacrifices individual staff made to make something possible.

21. \textbf{Lack of mediation in conflicts}\newline
Personal disputes linger on for a long time, potentially disrupting productivity, as there is no procedure or responsible person to mediate the two opposing parties. 
\subsection{Intrapersonal Challenges}
1. \textbf{Bad Work-Life-Balance}\newline
Unmitigated fatigue leading to less productivity during work hours.

2. \textbf{Work is not solution-oriented}\newline
A lot of time is spent on work that does not add to the solution, but is necessary to meet a certain (potentially emotional) expectation. Example: A certain style of code is required even though the delivered code meets quality and maintainability standards. An unsuitable framework is used because a team lead prefers it.

3. \textbf{Tasks insufficiently analyzed}\newline
The complexity and requirements of a task were not explored well enough, thus leading to an incorrect time assessment or lack of required knowledge to solve it well and in time.

4. \textbf{Task is not well defined or explained}\newline
Tasks are often not explained sufficiently, leave too much room for interpretation, possibly leading to unnecessary or wrong implementations that need to be revised later on.

5. \textbf{Lack of knowledge}\newline
The assigned tasks require far more expertise than the assignee has. While a challenging task can lead to growth, a task that is by far too difficult can hinder learning (Zone of proximal development).

6. \textbf{Gold Plating}\newline
Tasks are “overdone” and more functionality than required by the task or client is added.

7. \textbf{Demotivation}\newline
Time is wasted and procrastination occurs as there is a feeling of not wanting to work on specific tasks.
